# Supplementary material for: Autonomous Navigation in Unknown Environments using Sparse Kernel-based Occupancy Mapping
Source: arXiv:2002.01921 source file (2020-02-05)
Supplement: Supplementary file 1 [file Appendix.tex]

\appendices
\section*{APPENDICES}
\label{sec:appendix}

\subsection{Technical Approach}
%\label{subsec:technical_approach_appendix}
\subsubsection{Data Generation}
\label{app:data_gen}

\iffalse
\begin{figure}[h!]
\centering
\begin{subfigure}[t]{0.33\textwidth}
        \centering
        \includegraphics[height=1.65in]{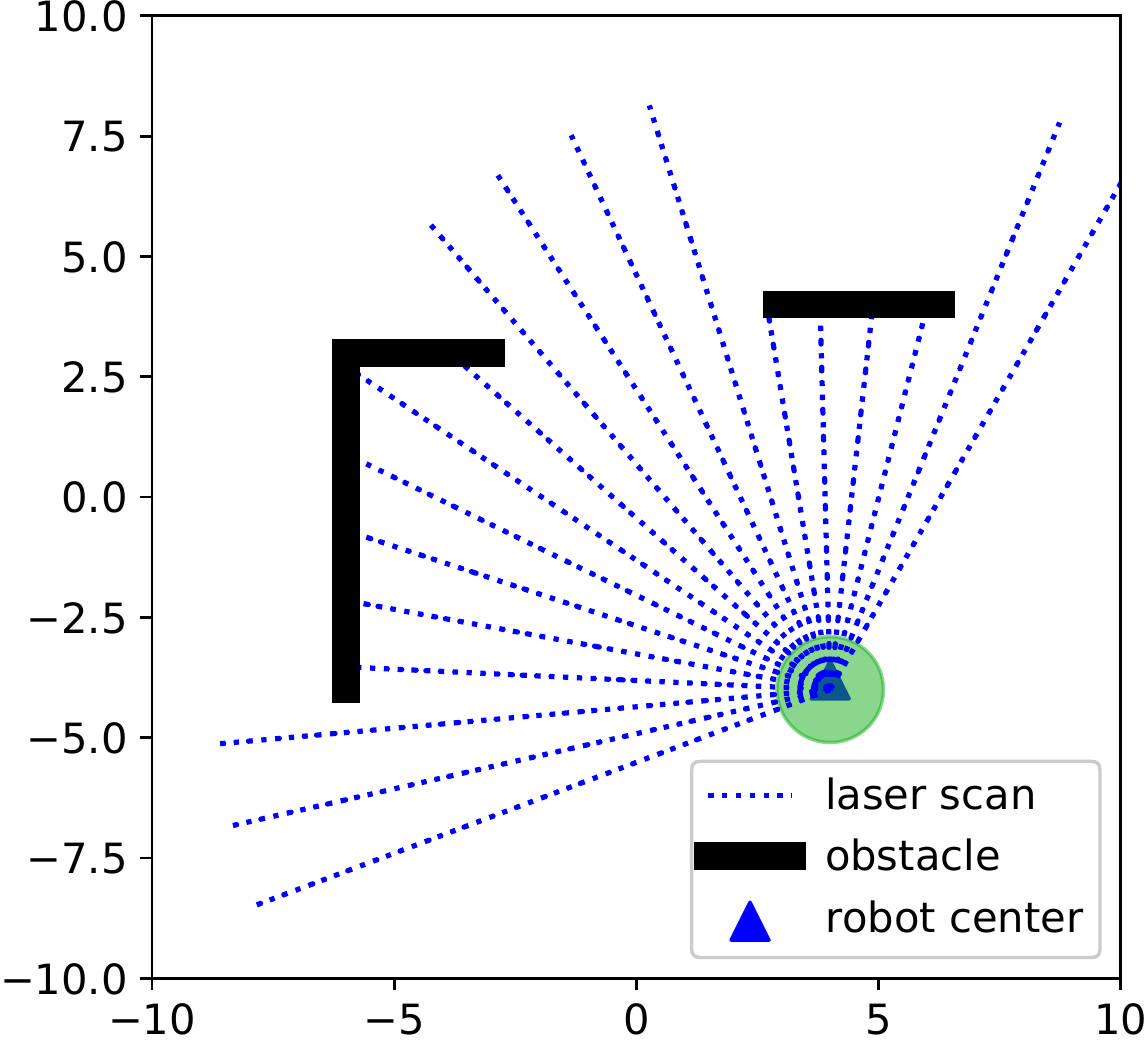}
        \caption{Depth scan in workspace.}
        \label{fig:laser_scan_ws}
\end{subfigure}%
\begin{subfigure}[t]{0.33\textwidth}
        \centering
        \includegraphics[height=1.65in]{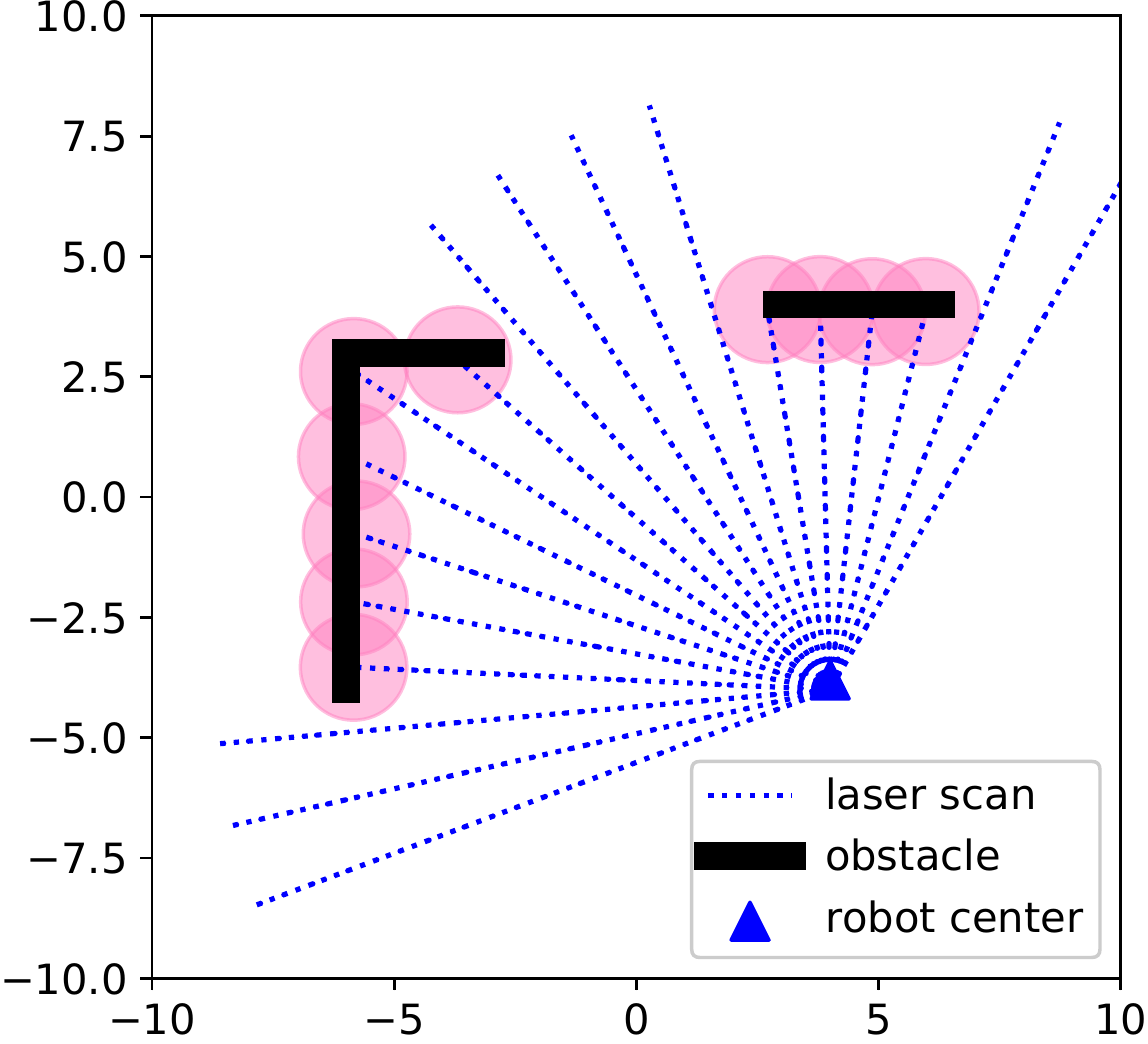}
        \caption{\centering Depth scan in C-space.}
        \label{fig:laser_scan_cs}
\end{subfigure}%
\begin{subfigure}[t]{0.33\textwidth}
        \centering
        \includegraphics[height=1.65in]{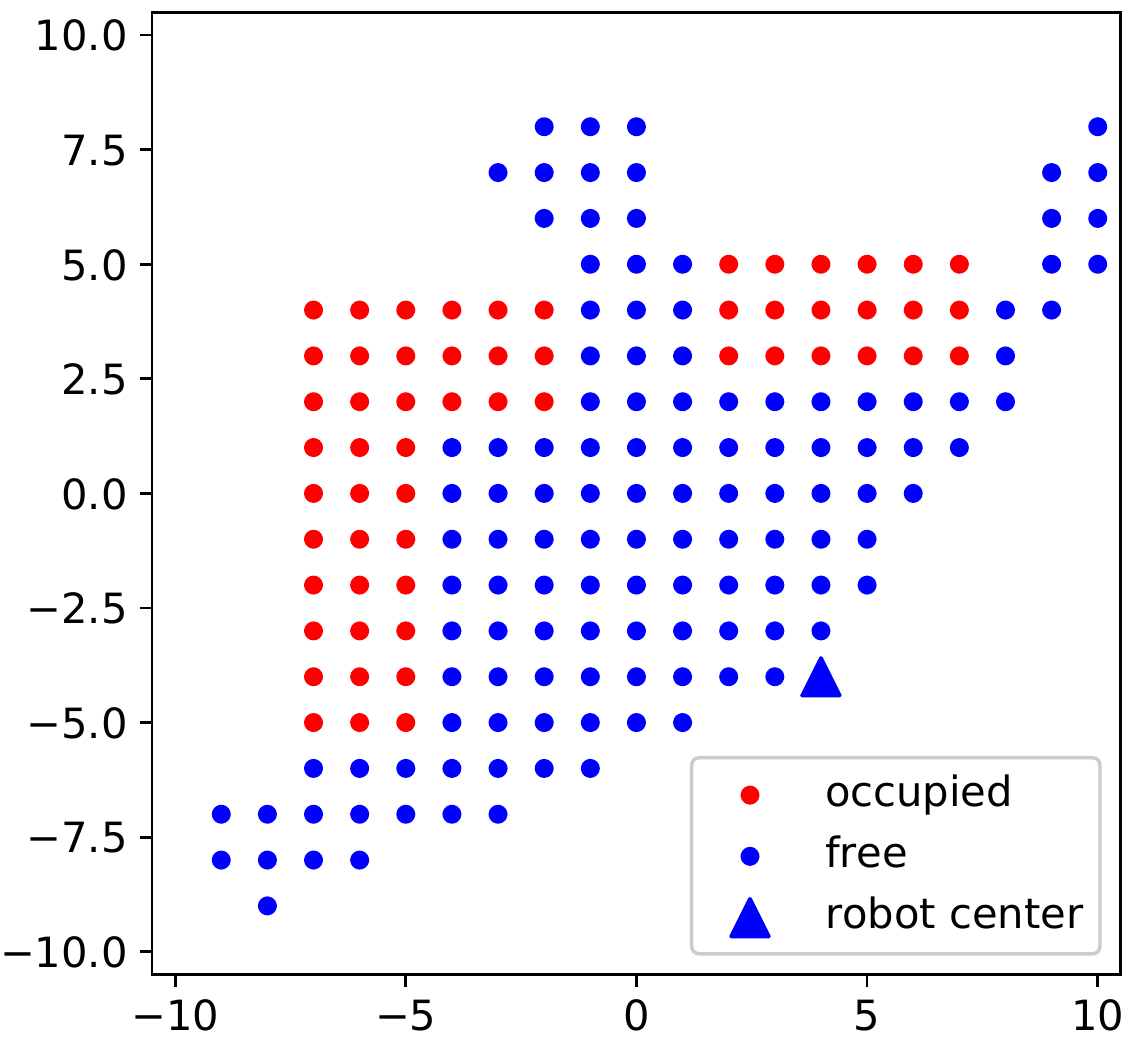}
        \caption{Samples from depth scan.}
        \label{fig:orig_data}
\end{subfigure}%
     
\begin{subfigure}[t]{0.33\textwidth}
        \centering
        \includegraphics[height=1.65in]{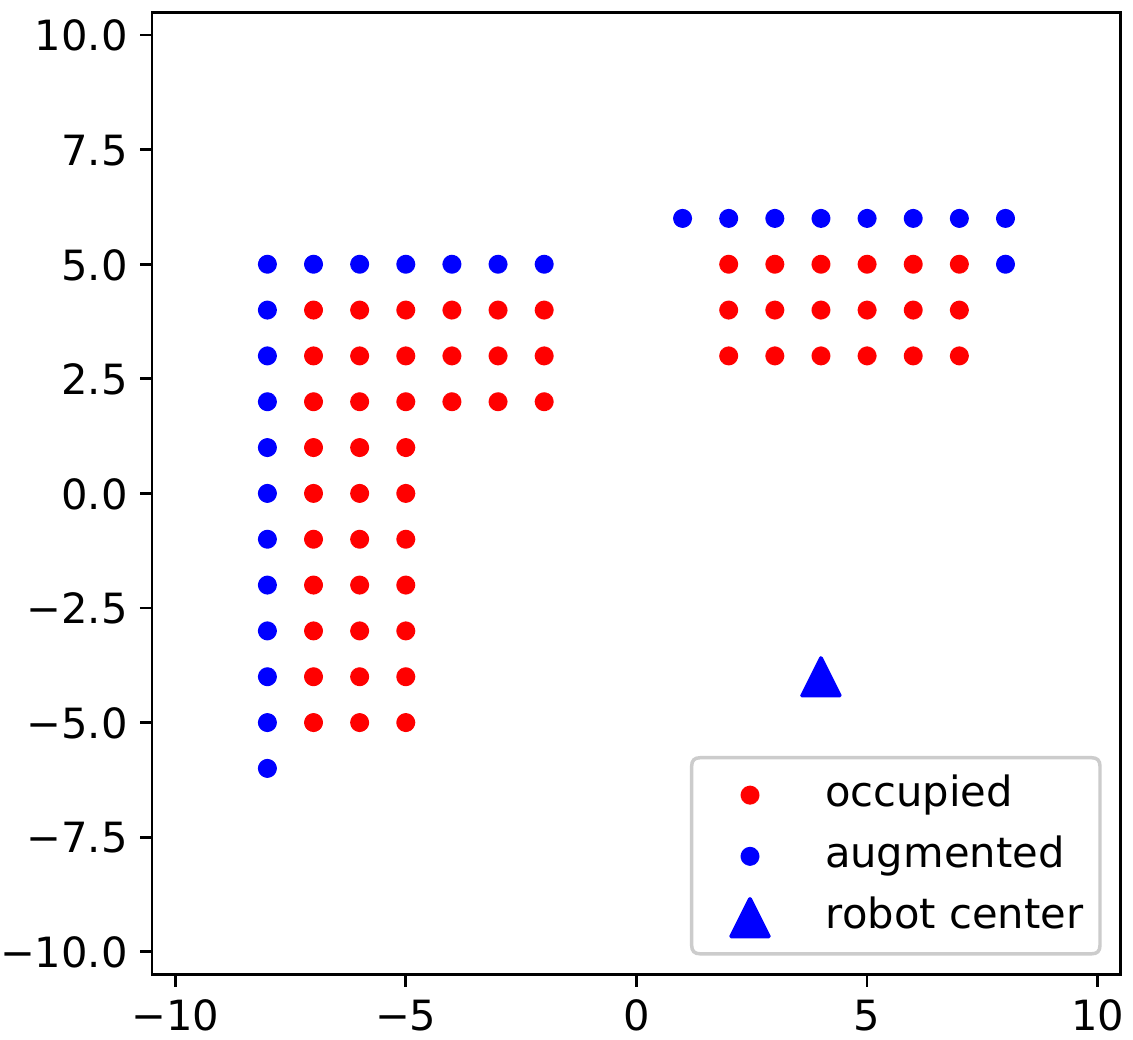}
        \caption{Augmented free points.}
        \label{fig:augmented_data}
\end{subfigure}%
\begin{subfigure}[t]{0.33\textwidth}
        \centering
        \includegraphics[height=1.65in]{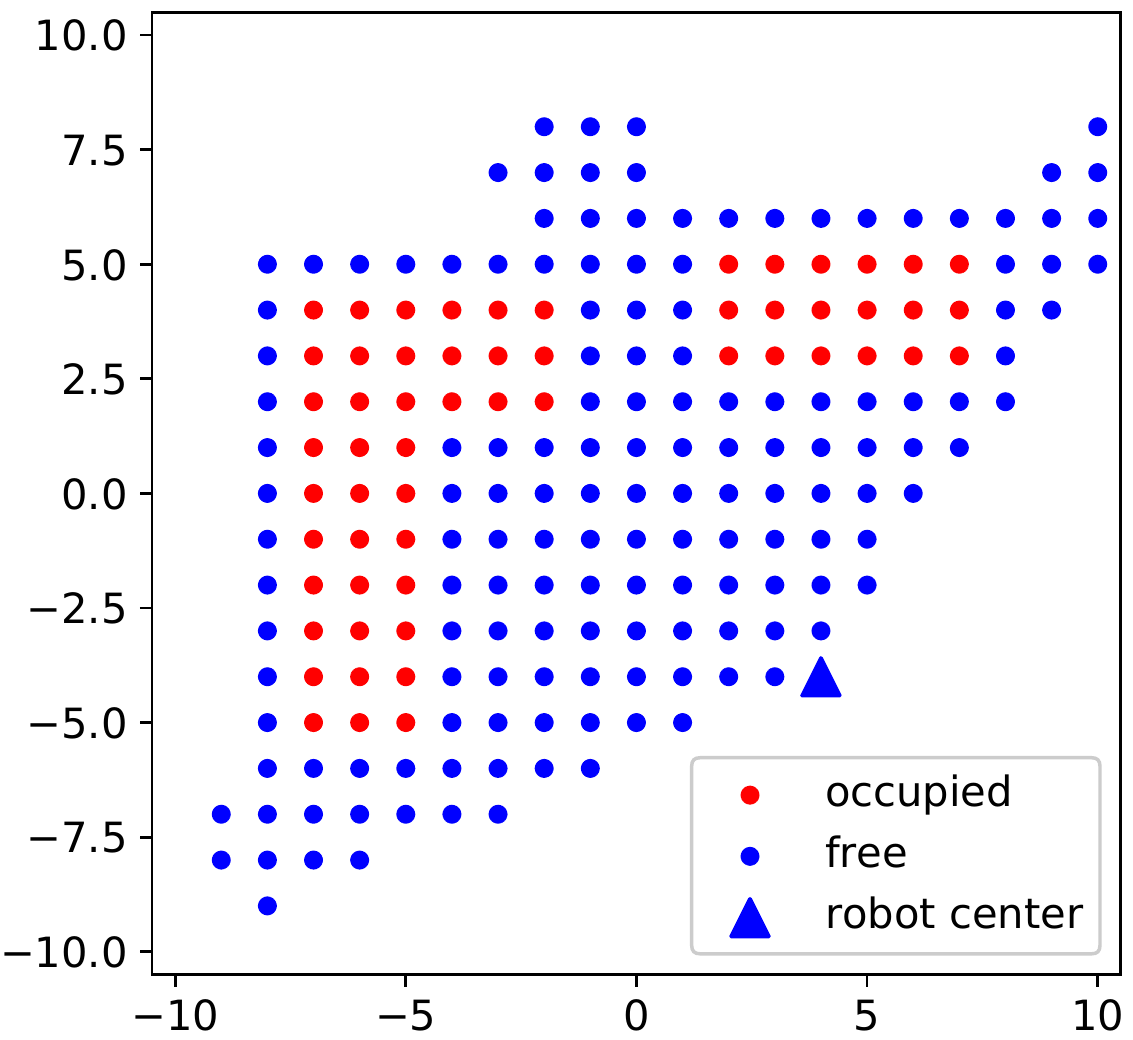}
        \caption{Training set $\mathcal{D}$}
        \label{fig:training_data}
\end{subfigure}%
\begin{subfigure}[t]{0.33\textwidth}
        \centering
        \includegraphics[height=1.65in]{fig/support_vecs_examples.pdf}
        \caption{Trained kernel perceptron model.}
        \label{fig:fastron_support_vectors}
\end{subfigure}%
\caption{Generation of a training dataset from a lidar scan and trained kernel perceptron model.}
\label{fig:fastron_example}
\end{figure}
\fi
The detailed algorithm for data generation in Section~\ref{subsec:ogm_with_fastron} is shown below.

\subsubsection{Collision Checking for Polynomial Curves}
\label{subsubsec:check_curves_appendix}

\subsection{Additional Experiment Results}

\subsubsection{Map Comparison}
\label{subsubsec:map_comparison_appendix}
Fig. \ref{fig:map_comparison_appendix} shows our simulation results for our kernel-based map, gmapping map, our inflated map generated by the upper bound proposed in Proposition.~\ref{prop:score_bounds}, and the resulting support vectors. Fig. \ref{fig:support_vec_count_appendix} shows that our kernel-based map stores 10 times less than gmapping does.

\subsubsection{Real Racecar Robot}
\label{subsubsec:real_car_appendix}
The support vectors, our kernel-based map and our inflated boundary generated by the upper bound in Proposition \ref{prop:score_bounds} are shown in Fig. \ref{fig:realcar_results_appendix}.

\begin{figure}[h!]
\centering
\begin{subfigure}[h!]{0.5\textwidth}
        \centering
        \includegraphics[width=\textwidth]{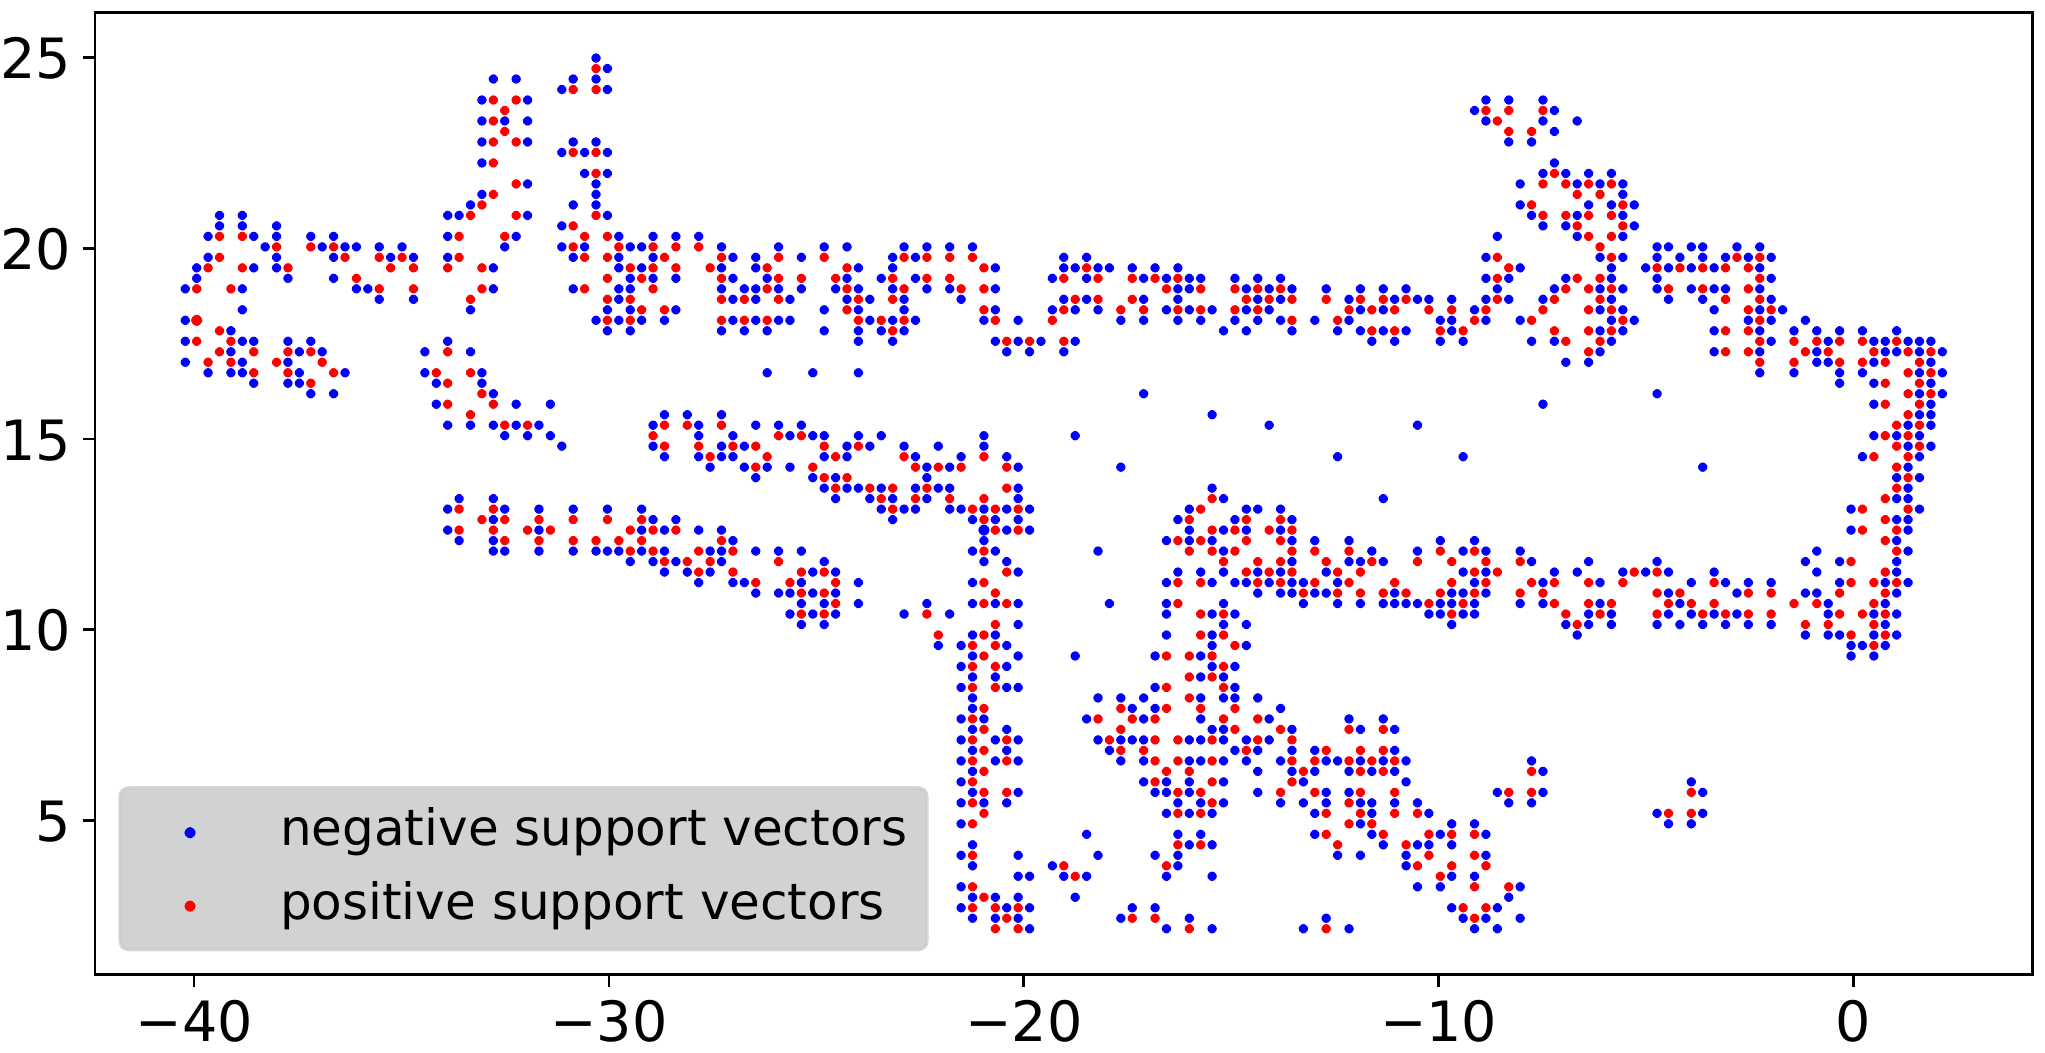}
        \caption{Support vectors maintained by our algorithm.}
        \label{fig:realcar_support_vec_appendix}
\end{subfigure}%

\begin{subfigure}[h!]{0.5\textwidth}
        \centering
        \includegraphics[width=\textwidth]{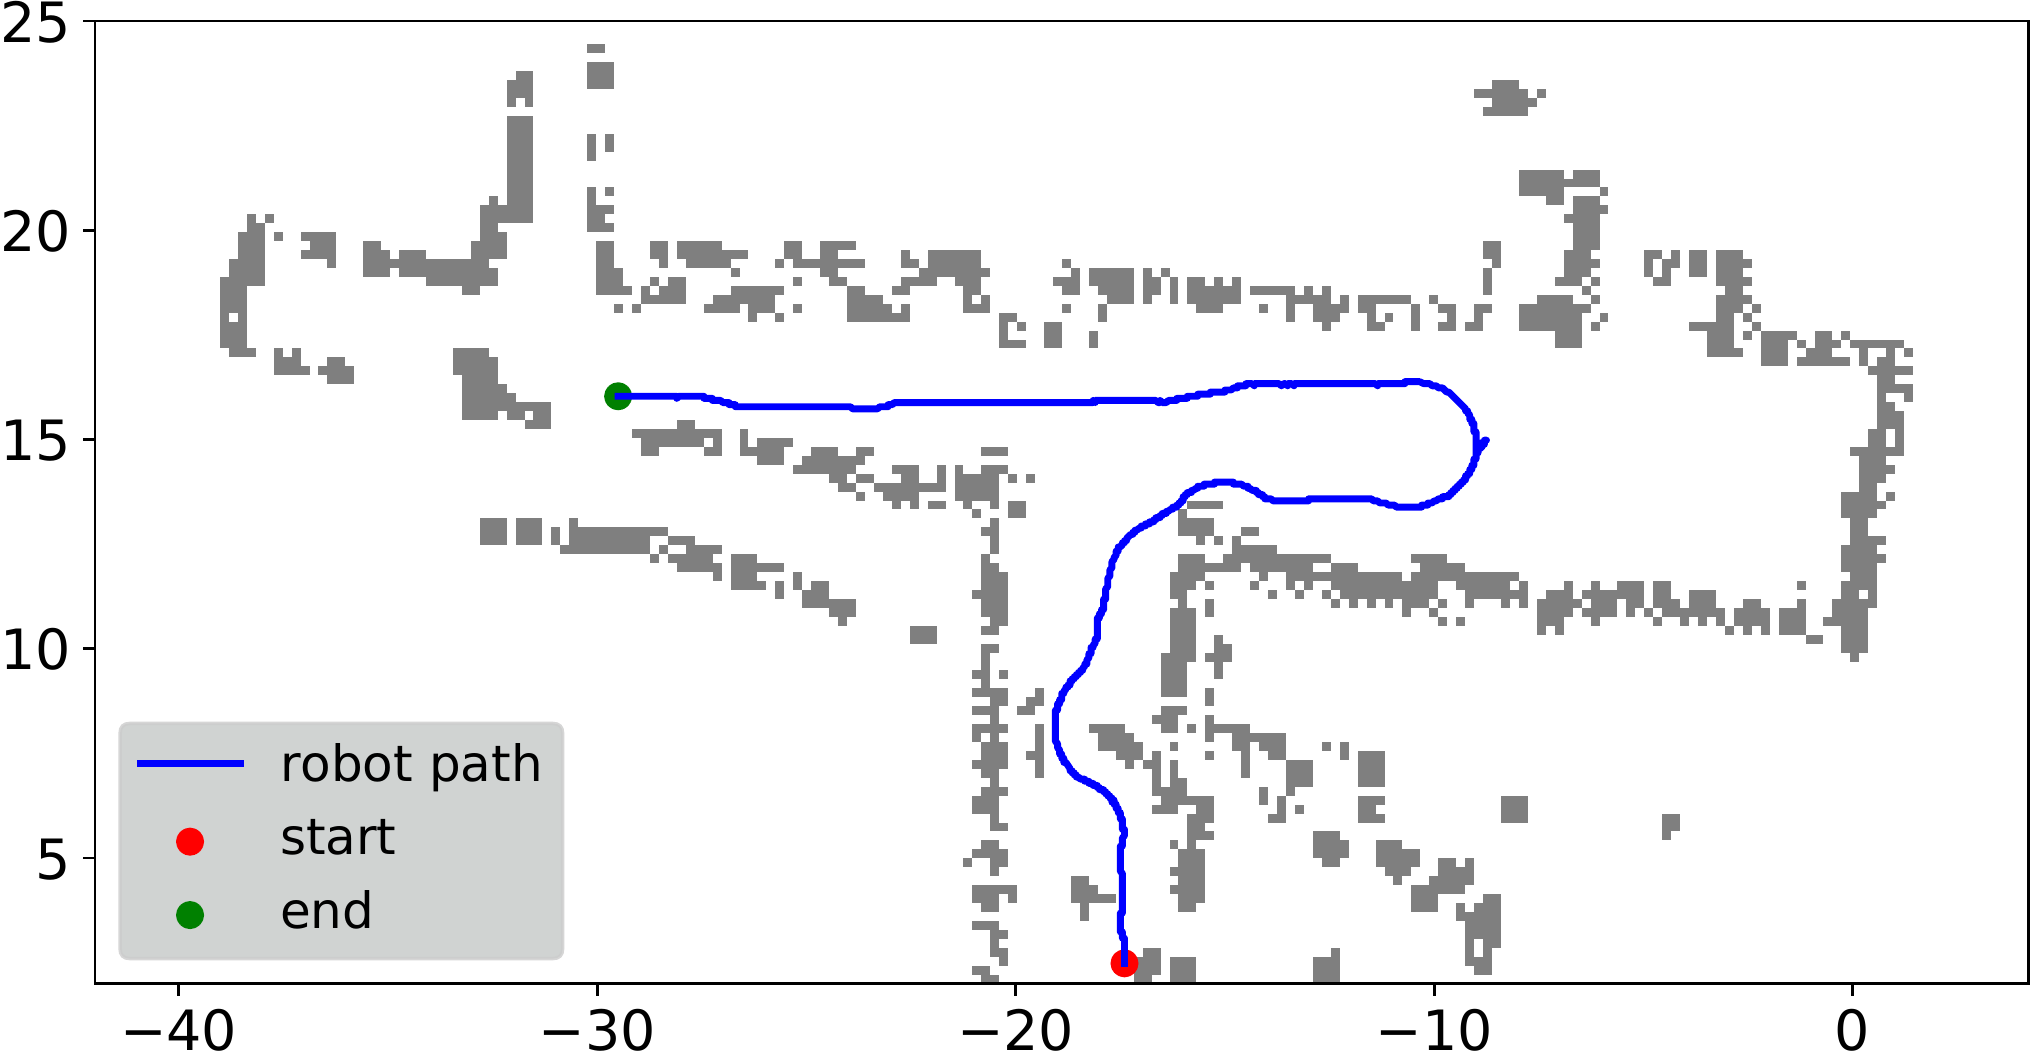}
        \caption{Kernel-based occupancy map.}
        \label{fig:realcar_final_map_appendix}
\end{subfigure}%

\begin{subfigure}[h!]{0.5\textwidth}
        \centering
        \includegraphics[width=\textwidth]{fig/realcar_upperbound.pdf}
        \caption{Occupancy map generated using the upper bound $U(x)$ proposed in Proposition~\ref{prop:score_bounds}.}
        \label{fig:realcar_upperbound_map_appendix}
\end{subfigure}%
\caption{Resulting maps generated by our mapping method.}
\label{fig:realcar_results_appendix}
\end{figure}
